# Supplementary material for: Further results on Minimal and Minimum Cylindrical Algebraic Decompositions
Source: arXiv:2601.09548 source file (2026-01-14)
Supplement: Supplementary file 1 [file Appendix.tex]

\appendix

\section{Analytic Trousers}

\red{Pour info:}

\begin{lemma}
The analytic trousers is the union of a smoothly embedded algebraic manifold $\tau$ and the half-line $\big\{(x, 0, 0) : x \geq 0 \big\}$. \\
\blue{The analytic Trousers $\mathbb{T}^\omega$ is the union of two analytic submanifolds of $\R^3$.} 
\end{lemma}

\begin{proof}
Consider the function \blue{$R$ ou $f$ ?} $R : \R^2 \setminus \{(x, 0) : x \geq 0\} \to \R$ defined by 
\[
f(x,y) = \sign(y)  \sqrt{\frac{x + \sqrt{x^2 + y^2}}{2}}. \red{check notations?}
\]
Then we have $\mathcal{G}(R) = \mathbb{T}^\omega \setminus \big\{(x, 0, 0) : x \geq 0 \big\}$. Indeed, let $(x,y) \in \R^2 \setminus \{(x, 0) : x \geq 0\}$. If $y = 0$, we find $x<0$ and $(x,y, f(x,y)) = (x,0,0) \in \mathbb{T}^{\omega}\setminus \big\{(x, 0, 0) : x \geq 0 \big\}$. If $y\neq 0$, setting $z = f(x,y)$ we first note that $$y z = |y|\sqrt{\frac{x + \sqrt{x^2 + y^2}}{2}} > 0$$ and then 
\[
4 z^4 - 4 z^2 x - y^2 = (x + \sqrt{x^2 + y^2})^2 - 2 (x+\sqrt{x^2 + y^2}) x + x^2 -(x^2 + y^2) = 0.
\]
Hence, we have shown $\mathcal{G}(R) \subset \mathbb{T}^\omega \setminus \big\{(x, 0, 0) : x \geq 0 \big\}$. To conclude, let $(x, y, z) \in \mathbb{T}^\omega \setminus \big\{(x, 0, 0) : x \geq 0 \big\}$. If $y=0$, we have $z = 0, x<0$ and hence $(x,y,z) \in \mathcal{G}(R)$ since in this case, we have $f(x,y,z) = 0$.  If $y\neq 0$, we deduce that $z$ is a solution of the biquadratic equation 
\[
4 z^4 - 4 z^2 x - y^2 = 0. 
\]
Since we have the condition $yz >0$, we conclude that $z = \sign(y)  \sqrt{\frac{x + \sqrt{x^2 + y^2}}{2}}$ and hence $(x,y,z) \in \mathcal{G}(R)$. To conclude, we observe that the function $(R\circ \phi)(r,\theta) =\sqrt{r} \cos\left(\frac{\theta}{2}\right)$ if $\phi(r, \theta) = (r\cos(\theta), r\sin(\theta))$ denotes  polar coordinates. Hence the function $R$ is analytic on its domain of defintion. 
\end{proof}
